# Supplementary material for: SmartBook: AI-Assisted Situation Report Generation for Intelligence Analysts
Source: arXiv:2303.14337 source file (2024-05-27)
Supplement: Supplementary file 1 [file appendix.tex]

\section{SmartBook Framework Details}
\label{sec:appendix}
Here we extend the description of the SmartBook framework from the paper's section~\ref{sec:smartbook} in terms of the various back-end workflow phases illustrated in Figure~\ref{fig:overall_workflow} for the automatic creation of situation reports.

Our automatic situation report is organized in the form of timelines to provide a coherent, chronological representation of event developments, facilitating users' tracking and understanding of the overall situation context. Each timeline spans a duration of 2 weeks, allowing for a manageable cycle of capturing and focused analysis of significant newsworthy occurrences.
Building upon this, major events are identified via clustering news articles within the 2-week timeline duration and serve as the foundation for corresponding chapters (details in section \ref{subsec:major_event}). To further guide detailed chapter analysis, we incorporate a logical structure through automatically generating section headings in the form of strategic questions relating to each major event (details in section \ref{subsec:section_headings}). SmartBook generates chapter content with strategic perspective by using such strategic questions covering various aspects of the event.
The individual sections comprise the core content of our situation report and contain grounded, query-focused summaries which address the strategic questions (details in section \ref{subsec:content_gen}), providing readers with a comprehensive understanding of event context and implications. 
The generated summaries feature citation linking, which grounds each summary fragment in its factual input context and allows experts to cross-check and verify information as needed.
Ultimately, the intuitive and structured incorporation of timeline chunking, major event chapter clustering, and query-focused section summaries within chapters enables our proposed SmartBook formulation to generate reliable, insightful reports for time-sensitive, emerging situations. 

\subsection{Major Events within Timespans as Chapters}\label{subsec:major_event}

For each timespan, we first identify major events within news article clusters during that time. 
To facilitate information navigation, we then introduce how to derive a high-level chapter name for each  event cluster, and use it as keyphrase to retrieve additional news articles for enriched situation report generation.

Our approach to identifying major events within a timespan begins with collecting news articles\footnote{Specifically, we use a running list of daily news snippets provided by CNN. For example \url{https://edition.cnn.com/europe/live-news/russia-ukraine-war-news-12-21-22/}} for a 2-week duration corresponding to the timeline. 
As the number of major events is unknown a priori, we cluster the daily news summaries into major event groups utilizing the agglomerative hierarchical clustering algorithm \cite{jain1988algorithms}, based on their term frequency-inverse document frequency (TF-IDF) scores, which assign higher weights to rare or document-specific words \cite{sparck1972statistical}.
Finally, we are left with clusters of news snippets, each providing a focused view to a major event. But because news summary snippets are condensed in detail, we want to enrich the comprehensiveness of major event cluster with chapter name and news corpus expansion, as detailed next.

%\subsubsection{Naming Chapters from Event Clusters}\label{subsubsec:name_chapters}
A key to further enriching event cluster representation is to derive a corresponding short chapter name, to facilitate information readability and retrieval, for the timeline within the situation report.
To achieve this, we utilize a sequence-to-sequence transformer-based \cite{vaswani2017attention} language model, BART \cite{lewis2020bart}, that has been trained on the NewsHead 
 dataset \cite{headline2020} for multi-document news headline generation. Each cluster within NewsHead contains up to five news articles and a crowd-sourced headline of up to 35 characters which describes the major information covered by the story in the cluster. Specifically, we take the concatenated title and text from all the news snippets within the event cluster as input sequences into the BART language model to generate a short event heading.
With the generated chapter name, we query google news to obtain an expanded set of news articles relevant to the event. In particular, we get news articles corresponding to the given timeline by formatting the query as follows, \textcolor{gray}{query = \textit{$<$Chapter name$>$ after:$<$Timeline start date$>$ before:$<$Timeline end date$>$}}, with start and end dates in the \textcolor{gray}{\textit{yyyy:mm:dd}} format.

\subsection{Strategic Questions as Section Headings}\label{subsec:section_headings}
Beyond simply describing event details in each major event chapter, SmartBook aims to provide information from a strategic perspective that can help aid decision-making and policy planning.
Thus, in this work, we generate chapter content with the use of questions that cover various strategic aspects of the event, which include  the possible motivations of the actors in an event and the future implications of the event. These strategic questions are organized in the form of section headings to incorporate structure into the chapter. As we detail next, the event-related questions are generated by prompting GPT-3 \cite{brown2020language}  
with a grounded context in the form of news articles from the event cluster. The generated questions then undergo a post-processing step of de-duplication to ensure clear and unique section headings. 

Recent work \cite{sharma2021generative, wang2022towards} has shown that GPT-3 is capable of generating natural questions that require long-form and informative answers, in comparison to existing approaches \cite{murakhovska-etal-2022-mixqg, du-etal-2017-learning} that mainly generate questions designed for short and specific answers. In this work, we prompt GPT-3 to explicitly generate strategic questions about the event. Further, to mitigate hallucinations \cite{ji2022survey, maynez2020faithfulness} which are common in large language models, we ground the input context to GPT-3 with news articles from the event cluster (from section \ref{subsec:major_event}) to ensure the generated questions are relevant to the event. Figure \ref{fig:overall_workflow} contains an example with the prompt used to generate strategic questions with GPT-3 for a chapter named \textit{Retreat of Russian Troops from Lyman}. News articles within the context are shown, with the prompt \hl{highlighted} in bold at the end. 
To ensure diversity in the generated questions, we sample multiple question sets from GPT-3 using nucleus sampling \cite{holtzman2019curious}.

Within the generated question sets, we observe that questions may sometimes be repeated across different sets. Figure  \ref{fig:overall_workflow} contains an example, with the duplicate questions within the generated question sets marked in \textcolor{blue}{blue}. The problem is similar to that of detecting duplicate question pairs given a large collection of questions. For this, we leverage a publicly available\footnote{\url{https://huggingface.co/cross-encoder/quora-roberta-large}} RoBERTa-large \cite{liu2019roberta} model trained on the Quora Duplicate Question Pairs\footnote{\url{https://quoradata.quora.com/First-Quora-Dataset-Release-Question-Pairs}} dataset. Given a pair of questions, the model predicts a score between 0 and 1 on how likely the two given questions are duplicate. We follow this approach for filtering out duplicate questions in order to merge the multiple question sets generated by GPT-3 into a single set of diverse and unique strategic questions about the event. 

\subsection{Extraction of Claims and Hypotheses}\label{subsec:claim_extraction}
Traditionally, a situation report requires foraging for different claims and hypotheses from the source documents (i.e., news articles) that help explain a situation \cite{toniolo2023human}, which is expensive to obtain through manual crowd-sourcing.
However, recent work \cite{reddy2022newsclaims, reddy2022zero} has shown that directed queries, such as strategic questions in our case, can be used to automatically extract claims from news articles relevant to a particular topic. Following our previous work\cite{reddy2022zero}, we adopt a Question Answering (QA) formulation to identify claims relevant to a given strategic question. Specifically, we design a QA pipeline, utilizing a transformer-based RoBERTa-large encoder model \cite{liu2019roberta} variant\footnote{We use the \href{https://huggingface.co/tasks/question-answering\#inference}{question-answering} pipeline provided by huggingface.} that has been trained on SQuAD 2.0 \cite{rajpurkar2018know} and Natural Questions \cite{kwiatkowski2019natural}. The pipeline takes as input the news corpus split into snippets along with the strategic question, and outputs short answer extractions to these questions. 
The identified short answers are then expanded, by including the 3-sentence window around it to provide additional context. 

However, there is still a risk of false positives \cite{tan2018know, chakravarti2021towards} being identified as candidate answers with high confidence, thus necessitating the validation \cite{reddy2020answer, zhang2021joint} of extracted answers. To this end, we employ an answer sentence selection model \cite{Garg_2020} that validates each of the extracted contexts (from Section \ref{subsubsec:claim_extraction}) separately against the strategic question. We concatenate the question and extracted context as input to a binary classification model\footnote{Model is available at \href{https://github.com/alexa/wqa_tanda\#tanda-models-transferred-on-asnq-then-fine-tuned-with-wiki-qa}{TANDA github}.}, with an underlying RoBERTa-large backbone, that is trained on Natural Questions \cite{kwiatkowski2019natural} and WikiQA \cite{yang-etal-2015-wikiqa}. The output of the model is a validation score, between 0 (incorrect answer selection) and 1 (correct answer selection), used to select the top-5 relevant contexts for summarization.

\subsection{Grounded Summaries as Section Content}\label{subsec:content_gen}
Using strategic questions obtained for each chapter as section {\textit{headings}}, we incorporate query-focused summarization to generate each section's {\textit{content}}. 
Given the set of relevant claim contexts for a strategic question, we aim to generate a concise summary as \textbf{section content} within SmartBook chapters. Observing that humans overwhelmingly prefer summaries from prompt-based large language models (LLMs) \cite{brown2020language, chowdhery2022palm} over models fine-tuned on article-summary pairs \cite{lewis2020bart, zhang2020pegasus, liu2022brio} due to better controllability and easier extension to novel scenarios \cite{goyal2022news, bhaskar2022zero, reddy2022sumren}, we leverage the Instruct-tuned 175B GPT-3 model (text-davinci-003) \cite{brown2020language, ouyang2022training} for zero-shot summarization.
Specifically, we concatenate the top-5 most relevant contexts (from Section \ref{subsec:claim_extraction}) as input, along with an instruction along the lines of \textit{``summarize the above, regarding $<$strategic question X$>$, with citations''}, to form the input prompt for the summary generation. It is noteworthy that the use of citations from the input text context in the language model prompting is novel and impactful, as it ensures the generated summary is accurate and trustworthy. Moreover, this approach also enables users to easily verify the summary information against sources used in the input.
